# Supplementary material for: The Color-Dual Fates of $F^3$, $R^3$, and $\mathcal{N}=4$ Supergravity
Source: arXiv:2203.03592 ancillary file (2023-10-07)
Supplement: Supplementary file 1 [file vectorDefinitions.pdf]

# Ancillary file for “The color-dual fate of $\mathcal{N}=4$ Supergravity”

JJM Carrasco, M Lewandowski, NH Pavao

For any questions, please contact:

*mail@nicpavao.com*

---

## some helper code

```
In[1]:= Get[
  "https://raw.githubusercontent.com/drjjmc/ampGraphTools_mma/master/ampGraphTools/
  ampGraphTools.m"]

Welcome to ampGraphTools, version 0.6,
a work in progress, but fairly simple implementation of
ideas in http://arxiv.org/abs/arXiv:1506.00974 and refs
therein. - dr.jjmc@gmail.com.

In[2]:= getPolRules[cut_, pols_] :=
  Reduce[Table[ulp[pol[[1]], pol] == 0, {pol, pols}] ~Join~ Table[
    ulp[pol, (tree /. Atree[a_] => Total[a])] == 0, {pol, pols}, {tree, cut}] //
  Flatten, Backsubstitution -> True] // ToRules
```

```

In[3]:= refreshGRAPHRULES :=
  (Clear[graphAlgRules];
   graphAlgRules[g_] :=
     graphAlgRules[g, {}];
   graphAlgRules[gness_, hold_] := Module[{rules, g, eqns},
     g = gness /. massive[in[x_], b_] => in[massive[x, b]];
     eqns = g /.
       vertexFormGraph[necklaces_] => necklaces /.
       neckl[a_] => Plus@@a == 0;
     rules = (ToRules@ Reduce[eqns,
       Complement[extractType[g, in] // Union, hold],
       Backsubstitution -> True]);
     Select[rules, Head[#1] ~SameQ~ in &] /.
     Flatten[Map[{#, -#[1] -> -#[2]} &, (Reverse /@
       Select[rules, Head[#1] ~UnsameQ~ in &))]] /.
     in[massive[x_, b_] => massive[in[x], b] ];)
refreshGRAPHRULES

In[5]:= getIndepReq[treeList_, req_] := Module[{me, legs, loops, doo, eqns2, Subscript,
  myTrees = treeList, eqns,
  free =
    Flatten[{List @@ Expand[req /. uLsq[{a_, b_}] => ulp[a, b] /. -1 => 1]}],
  ks}, Subscript[a_, b_] := a[b];
  legs = Union[Flatten[myTrees /. Atree[a_] => a /. -(a_) => a]];
  loops = Select[legs, #1[[1]] === l &]; ks = Select[legs, #1[[1]] === k &];
  doo = Union[Flatten[Outer[ulp[#1, #2] &, legs, legs] ]];
  doo = Complement[doo, free]; eqns = myTrees /. Atree[a_] => Plus @@ a;
  eqns2 = Flatten[{(me = #1; (ulp[#1, me] == 0 &) /@ eqns) &} /@ legs] ~Join~ (
    ulp[#, #] == 0 & /@ legs); Reduce[eqns2, doo, Backsubstitution -> True]

```

```

In[6]:= graphBasisRules[graph_] := Module[{cons, vs, eqns, solveFor, ext, legs, badGuy},
  cons = graph[[1]] /. neckl[a_] => Plus @@ a;
  ext = getExtLegs[graph]; badGuy = First@Complement[ext, getMyUniqLegs[graph]];
  legs = graph[[1]] /. neckl => List /. -a_ => a // Flatten // Union;
  vvsGBR = vs = Join[
    Union[
      Flatten[
        Table[{ulp[#1, con] == 0 & } /@ legs, {con, cons}]
      ]
    ],
    {ulp[#1, #1] == 0 & } /@ ext]; zsf =
  solveFor = Sort[Select[Union[extractType[vs, ulp]], Position[#, badGuy] != {} ||
    Position[#1, in] != {} || Position[#1, l] != {} &],
    OrderedQ[{#1, #2} /. ulp => Times /. Map[# -> 10 &, getMyUniqLegs[graph]] /.
      k[_] => 5 /. l[___] => 2 /. in[___] => 0] &];
  ToRules[Reduce[vs, solveFor, Backsubstitution -> True]]]

In[7]:= defRules[graph_] := Module[{myLegs, myLoops, myCutMass, myMasslessGuys,
  myExtLegs, myPols, dotRules, myPolRules, LEGS, myBasisRules, simpRules,
  masslessLegs, graphObj},
  myExtLegs = getExtLegs[graph];
  LEGS = Length[myExtLegs];
  masslessLegs = myExtLegs;
  simpRules = Table[-Total@voosh -> First@Complement[myExtLegs, voosh],
    {voosh, Subsets[myExtLegs, {LEGS - 1}]}];
  dotRules = graphBasisRules[graph];
  myPolRules =
    getPolRules[Join[{Atree[myExtLegs]}, consistentGraphToTrees[graph]],
      # /@ masslessLegs];
  graphObj["dotRules"] = dotRules;
  graphObj["myPolRules"] = myPolRules;
  graphObj["simpRules"] = simpRules;
  graphObj]

In[8]:= expandBasis[expr_, graph_] := Module[{myLegs, myLoops, myCutMass,
  myMasslessGuys, myExtLegs, myPols, dotRules, myPolRules, LEGS,
  myBasisRules, simpRules, masslessLegs, myGraphObj},
  myGraphObj = defRules[graph];
  simpRules = myGraphObj["simpRules"];
  dotRules = myGraphObj["dotRules"];
  myPolRules = myGraphObj["myPolRules"];
  expr //. Reverse[First[simpRules]] //. dotRules //. simpRules //. dotRules //.
    myPolRules]

```

```

In[9]:= graphCutBasisRules[graph_] :=
Module[{cons, vs, eqns, solveFor, ext, legs, badGuy},
  cons = graph[[1]] /. neckl[a_] => Plus @@ a;
  ext = (graph~extractType~neckl) /. neckl[a_] => a /. -a_ => a // Flatten // Union;
  badGuy = First@Complement[ext, getMyUniqLegs[graph]];
  legs = graph[[1]] /. neckl => List /. -a_ => a // Flatten // Union;
  vvsGBR = vs = Join[
    Union[
      Flatten[
        Table[{ulp[#1, con] == 0 & } /@ legs, {con, cons}]
      ]
    ],
    ({ulp[#1, #1] == 0 & } /@ ext]; zsf =
  solveFor = Sort[Select[Union[extractType[vs, ulp]], Position[#, badGuy] != {} ||
    Position[#1, in] != {} || Position[#1, l] != {} &],
    OrderedQ[{#1, #2} /. ulp => Times /. Map[# -> 10 &, getMyUniqLegs[graph]] /.
      k[_] => 5 /. l[___] => 2 /. in[___] => 0] &];
  ToRules[Reduce[vs, solveFor, Backsubstitution -> True]]]

In[10]:= defCutRules[graph_] := Module[{myLegs, myLoops, myCutMass, myMasslessGuys,
  myExtLegs, myPols, dotRules, myPolRules, LEGS, myBasisRules, simpRules,
  masslessLegs, graphObj},
  myExtLegs = getExtLegs[graph];
  LEGS = Length[myExtLegs];
  masslessLegs = myExtLegs;
  simpRules = Table[-Total@voosh -> First@Complement[myExtLegs, voosh],
    {voosh, Subsets[myExtLegs, {LEGS - 1}]}];
  dotRules = graphCutBasisRules[graph];
  myPolRules =
    getPolRules[Join[{Atree[myExtLegs]}, consistentGraphToTrees[graph]],
      e /@ masslessLegs];
  graphObj["dotRules"] = dotRules;
  graphObj["myPolRules"] = myPolRules;
  graphObj["simpRules"] = simpRules;
  graphObj]

```

```

In[11]:= expandCutBasis[expr_, graph_] :=
  Module[{myLegs, myLoops, myCutMass, myMasslessGuys,
    myExtLegs, myPols, dotRules, myPolRules, LEGS,
    myBasisRules, simpRules, masslessLegs, myGraphObj},
    myGraphObj = defCutRules[graph];
    simpRules = myGraphObj["simpRules"];
    dotRules = myGraphObj["dotRules"];
    myPolRules = myGraphObj["myPolRules"];
    expr //. Reverse[First[simpRules]] //. dotRules //. simpRules //. dotRules //.
    myPolRules]

In[12]:= easyBasisSolve[expr_] := basisSolve[expr, Union[extractType[expr, ulp]]]

In[13]:= basisEqnsNoEq[expr_, basis_] :=
  Last /@ Flatten[ArrayRules /@ Rest[CoefficientArrays[expr, basis]]]

In[14]:= basisEqns[expr_, basis_] := (#1 == 0 &) /@ basisEqnsNoEq[expr, basis]

In[15]:= basisSolve[expr_, basis_] := If[expr === 0, {},
  ToRules[(Reduce[#1, Union[extractType[#1, a]], Backsubstitution -> True] &)[
    basisEqns[expr, basis]]]]

In[16]:= doSomeGlueSewingBrute[expr_] := Module[{q}, q = qCrazyNoExcusesRef;
  expr //. {ulp[μ_, ε[-p_]] * ulp[ν_, ε[p_]] =>
    (ulp[μ, ν] -  $\frac{ulp[q, μ] \times ulp[p, ν] + ulp[p, μ] \times ulp[q, ν]}{ulp[q, p]}$ ) //.
    {ulp[ε[-aaa_], ε[aaa_]] => (Ds - 2), ulp[q, q] -> 0}} // ExpandAll]

```

---

## spanning set of building blocks: from 2104.08370

We will use  $\epsilon$  for polarization instead of  $\varepsilon$ . Simplest to just load in a block:

```

In[17]:= Block[{ε = ε},
  Get["https://raw.githubusercontent.com/sunazekioglu/fivePointEFT/main/
    fourPointVectorDressings.wl"]];

```

See results guide, fourPointResultsGuide.nb,

at <https://github.com/sunazekioglu/fivePointEFT>

as well as associated paper, <https://inspirehep.net/literature/1859154>, for details.

---

## Lining up 4-point vector building blocks ( $n^{0_i}$ ) with 1910.12850 reproduction of B(1234)

Below we construct the vector building blocks appearing in our paper from those previously constructed in the ancillary file of 2104.08370. The provided vector building blocks are in terms of functional numerator weights for the s-channel graph,  $n_s$ , grouped by order of monomial of Lorentz Products. First, we factor out an overall normalization:

```
In[18]:= relativeNorm = {a["(DF)^4_1"] → 8, a["(DF)^4_2"] → 8, a["(DF)^4_(2F^3+F^4)"] → 8,
  a["2F^3+F^4"] → 8, a["F^3"] → 8, a["D^2F^4_f^3"] → 8, a["YM"] → 8, a[mD[6], 1] → 8};
```

And define variables for spanning scalar permutation invariants, and  $\sigma_2 \propto (s^2 + t^2 + u^2)$ ,  $\sigma_3 \propto s t u$

```
In[19]:=  $\sigma3eval = ulp[k[1], k[2]] \times ulp[k[2], k[3]] \times ulp[k[1], k[3]]$ ;
```

```
In[20]:=  $\sigma2eval = (ulp[k[1], k[2]]^2 + ulp[k[1], k[3]]^2 + ulp[k[3], k[2]]^2) / 2$ ;
```

The `vec4num[monOrder]` function defined in the ancillary file returns the dressing of an s-channel graph labeled:

$\{k[1], k[2], i[1]\}, \{-i[1], k[3], k[4]\}$  that is order ‘monOrder’ in monomials of dot products. We represent dot products with the unevaluated Lorentz product head, `ulp`, as `ulp[a, b]` would mean  $a \cdot b$ .

We annotate the vector blocks which appear in our paper as follows:

$$n_s^{YM} = neval["YM"]$$

$$n_s^{YM+F^3} = neval["YM+F^3"]$$

and so forth.

```
In[21]:= neval["YM"] = vec4num[3] /. a["ym"] → a["YM"] /. relativeNorm;
(* Mass Dimension (MD) of YM *)
```

```
In[22]:= neval["YM+F^3"] =
  vec4num[4] /. {a[mD[4], 1] → 0, a[mD[4], 2] → 0, a["f^3"] → a["F^3"]} /.
  relativeNorm; (* MD ap over YM *)
```

```
In[23]:= neval["2F^3+F^4"] = vec4num[5] /. a[mD[5], _] → 0 /. a["2f^3+f^4"] → a["2F^3+F^4"] /.
  relativeNorm; (* MD ap^2 over YM *)
```

```
In[24]:= neval["D^2F^4"] = vec4num[6] -  $\sigma2eval$  vec4num[4] /.
  {a[mD[4], 1] → 0, a[mD[4], 2] → 0, a["f^3"] → a["D^2F^4_f^3"],
  a[mD[6], 1] → a["D^2F^4"]} /. relativeNorm; (* MD ap^3 over YM *)
```

```
In[25]:= neval["(DF)^4_1"] =
  - $\sigma3eval$  vec4num[4] -  $\sigma2eval$  vec4num[5] /. {a["f^3"] → 0, a[mD[4], 2] → 0,
  a[mD[4], 1] → a["(DF)^4_1"], a["2f^3+f^4"] → a["(DF)^4_(2F^3+F^4)"],
  a[mD[5], 3] → 0, a[mD[5], 4] → 0} /. relativeNorm; (* MD ap^4 over YM *)
```

```
In[26]:= neval["(DF)^4_2"] =  $\sigma3eval$  vec4num[4] /.
  {a["f^3"] → 0, a[mD[4], 1] → 0, a[mD[4], 2] → a["(DF)^4_2"]} /.
  relativeNorm; (* MD ap^4 over YM *)
```

The other two building blocks in the local spanning basis, up to powers of scalar permutation invari-

ants, are not required in this calculation, at least not through  $O(\alpha'^4)$

```
In[27]:= notUsed1 = Coefficient[vec4num[5], a[mD[5], 3]]; (* MD  $\alpha'^2$  over YM *)
```

```
In[28]:= notUsed2 = Coefficient[vec4num[5], a[mD[5], 4]]; (* MD  $\alpha'^2$  over YM *)
```

A spanning four-point color-dual numerator ansatz through mass dimension consistent with  $(\alpha')^4$  over YM would be as follows:

```
In[29]:= nSpanningThrough4aboveYM = vec4num[3] +  $\alpha'$  vec4num[4] +
   $\alpha'^2$  (vec4num[5] +  $\sigma$ 2eval (vec4num[3] /. a[x___]  $\Rightarrow$  a[x,  $\sigma$ 2])) +
   $\alpha'^3$  (vec4num[6] +  $\sigma$ 2eval (vec4num[4] /. a[x___]  $\Rightarrow$  a[x,  $\sigma$ 2]) +
   $\sigma$ 3eval (vec4num[3] /. a[x___]  $\Rightarrow$  a[x,  $\sigma$ 3])) +
   $\alpha'^4$  ( $\sigma$ 2eval (vec4num[5] /. a[x___]  $\Rightarrow$  a[x,  $\sigma$ 2]) +
   $\sigma$ 3eval (vec4num[4] /. a[x___]  $\Rightarrow$  a[x,  $\sigma$ 3]));
```

This involves 19 parameters:

```
In[30]:= nSpanningThrough4aboveYM ~ extractType ~ a
```

```
Out[30]:= {a[2f^3+f^4], a[f^3], a[ym], a[2f^3+f^4,  $\sigma$ 2], a[f^3,  $\sigma$ 2],
  a[f^3,  $\sigma$ 3], a[ym,  $\sigma$ 2], a[ym,  $\sigma$ 3], a[mD[4], 1], a[mD[4], 2],
  a[mD[5], 3], a[mD[5], 4], a[mD[6], 1], a[mD[4], 1,  $\sigma$ 2], a[mD[4], 1,  $\sigma$ 3],
  a[mD[4], 2,  $\sigma$ 2], a[mD[4], 2,  $\sigma$ 3], a[mD[5], 3,  $\sigma$ 2], a[mD[5], 4,  $\sigma$ 2]}
```

The ordered three-point amplitude labeled  $k/@\text{Range}[3]$  for the YM +  $\text{tr}F^3$  theory has the following antisymmetric kinematic numerator:

```
In[31]:= threePointDressing = 2  $\alpha'$  ulp[k[2],  $\epsilon$ [k[3]]]  $\times$  ulp[k[3],  $\epsilon$ [k[1]]]  $\times$  ulp[k[3],  $\epsilon$ [k[2]]] -
  2 ulp[k[2],  $\epsilon$ [k[3]]]  $\times$  ulp[ $\epsilon$ [k[1]],  $\epsilon$ [k[2]]] + 2 ulp[k[3],  $\epsilon$ [k[2]]]  $\times$ 
  ulp[ $\epsilon$ [k[1]],  $\epsilon$ [k[3]]] - 2 ulp[k[3],  $\epsilon$ [k[1]]]  $\times$  ulp[ $\epsilon$ [k[2]],  $\epsilon$ [k[3]]];
```

Which we can sew together over the physical gluon state projector to get the contribution to the “t”-channel cut.

We will need to enforce conservation of cut momenta etc, and create a function to do so:

```
In[32]:= tCut = {Atree[{k[2], k[3], -l[1]}], Atree[{l[1], k[4], k[1]}]};
```

```
In[33]:= cutBasis[expr_] := expr ~ expandCutBasis ~ (toGraph@tCut)
```

and perform the sewing with the projector defined above,

```
In[34]:= sewnTChannelCut = FixedPoint[doSomeGlueSewingBrute, Times@@ (tCut /.
  Atree[a__]  $\Rightarrow$  (threePointDressing /. Thread[Rule[k/@Range[3], a]])) //
  cutBasis // ExpandAll] // cutBasis // Collect[#,  $\alpha'$ , FullSimplify] &;
```

Let’s make a quick function to generate an ordered s, t, channel tree from a functional s-channel numerator:

```
In[35]:= basisFour[expr_] := expr ~ expandBasis ~ (vertexFormGraph[{neckl[k/@Range[4]]}])
```

```
In[36]:= nDots4 = Map[#  $\rightarrow$  RandomPrime[{10^3, 10^6}] &,
  ((vec4num/@Range[3, 7]) // basisFour) ~ extractType ~ ulp];
```

```
In[37]:= ampSTfromSNum[sNum_] := 
$$\frac{sNum}{2 \text{u}\ell p[k[1], k[2]]} + \left( (* \text{ t channel} *) \right. \\ \left. \frac{sNum}{2 \text{u}\ell p[k[1], k[2]]} /. \text{Thread}[\text{Rule}[k / @ \text{Range}[4], k / @ \{2, 3, 4, 1\}]] \right) // \text{basisFour}$$

```

So our ansatz ordered amplitude in the s-t channel is as follows:

```
In[38]:= ansatzAmp = ampSTfromSNum[nSpanningThrough4aboveYM];
```

To enforce factorization consistency on our color-dual ansatz, its' sufficient to consider this amplitude's residue on the t channel, under conservation of momenta associated with the cut.

```
In[39]:= cutAnsatz = Residue[ansatzAmp /. ulp[k[2], k[3]] -> t / 2, {t, 0}];
```

```
In[40]:= cutConstraints = {cutAnsatz - sewnTChannelCut // cutBasis // easyBasisSolve}[[2]]
```

```
Out[40]= {a[2f^3+f^4] -> 8, a[f^3] -> 8, a[ym] -> 8, a[2f^3+f^4, sigma2] -> 0, a[f^3, sigma2] -> 0, \\ a[ym, sigma2] -> 0, a[mD[4], 1] -> 0, a[mD[4], 2] -> 0, a[mD[5], 3] -> 0, a[mD[5], 4] -> 0, \\ a[mD[4], 1, sigma2] -> 0, a[mD[4], 2, sigma2] -> 0, a[mD[5], 3, sigma2] -> 0, a[mD[5], 4, sigma2] -> 0}
```

We see this is can be expressed in terms of our above normalized n-vector building blocks, eq (12), in the paper:

```
In[41]:= nFactorizingAnsatzThrough4 = n["YM"] + ap n["YM+F^3"] + ap^2 n["2F^3+F^4"] + \\ ap^3 (a[3] (n["D^2F^4"] + sigma2 n["YM+F^3"]) + \\ a[3, "YM"] sigma3 n["YM"]) + \\ ap^4 (a[4] (n["(DF)^4_1"] + sigma2 n["2F^3+F^4"]) + a[4, 2] x n["(DF)^4_2"] + \\ a[4, "F^3"] sigma3 n["YM+F^3"])
```

```
Out[41]= ap^2 n[2F^3+F^4] + n[YM] + ap n[YM+F^3] + \\ ap^4 (a[4] (sigma2 n[2F^3+F^4] + n[(DF)^4_1]) + a[4, 2] x n[(DF)^4_2] + \\ sigma3 a[4, F^3] x n[YM+F^3]) + ap^3 (sigma3 a[3, YM] x n[YM] + a[3] (n[D^2F^4] + sigma2 n[YM+F^3]))
```

```
In[42]:= ((nFactorizingAnsatzThrough4 /. {sigma2 -> sigma2eval, sigma3 -> sigma3eval, n -> neval}) - \\ (nSpanningThrough4aboveYM /. cutConstraints) // \\ basisFour) // easyBasisSolve // List // First
```

```
Out[42]= {a[f^3, sigma3] -> 8 a[4, F^3], a[ym, sigma3] -> 8 a[3, YM], \\ a[mD[6], 1] -> 8 a[3], a[mD[4], 1, sigma3] -> -8 a[4], a[mD[4], 2, sigma3] -> 8 a[4, 2]}
```

Upon fixing to factorization and color-kinematics satisfaction of a generic five-point ansatz through  $O(\alpha'^4)$ , we found the following constraints (eqs 13-15):

```
In[43]:= fivePointConstraints = {a[4, "F^3"] -> 1 + a[3, "YM"], \\ a[3] -> 1, a[4] -> 1, a[4, 2] -> 1}
```

```
Out[43]= {a[4, F^3] -> 1 + a[3, YM], a[3] -> 1, a[4] -> 1, a[4, 2] -> 1}
```

giving us the tower of higher-derivative contacts through  $O(\alpha'^4)$  at four points,



```
In[44]:= ndcc = nFactorizingAnsatzThrough4 /. fivePointConstraints //
Collect[#, {n[___]}, FullSimplify] &
```

```
Out[44]= (αp2 + αp4 σ2) n[2F3+F4] + αp3 n[D2F4] + αp4 n[(DF)41] + αp4 n[(DF)42] +
(1 + αp3 σ3 a[3, YM]) n[YM] + (αp + αp3 σ2 + αp4 σ3 (1 + a[3, YM])) n[YM+F3]
```

With the definition:

```
In[45]:= neval["(DF)^4"] = neval["(DF)^4_1"] + neval["(DF)^4_2"];
```

We find this consistent with the low order \alpha' expansion of (DF)<sup>2</sup>+YM amplitudes supplemented by free permutation invariants.

First we write the tachyonDenominator:

```
In[46]:= tachyonDenom = (1 - αp2 σ2 - αp3 σ3)-1
```

```
Out[46]= 
$$\frac{1}{1 - \alpha p^2 \sigma_2 - \alpha p^3 \sigma_3}$$

```

It's not so hard to see:

```
In[47]:= tachyonDenom -
((1 - αp ulp[k[1], k[2]]) (1 - αp ulp[k[2], k[3]]) (1 - αp ulp[k[1], k[3]]))-1 /.
{σ2 → σ2eval, σ3 → σ3eval} // basisFour // FullSimplify
```

```
Out[47]= 0
```

that this is equivalent to:  $((1 - \alpha' k_1 \cdot k_2)(1 - \alpha' k_2 \cdot k_3)(1 - \alpha' k_1 \cdot k_3))^{-1}$

We reproduce the expression for n["DF<sup>2</sup>+YM"]

```
In[48]:= n["DF^2+YM"] = n["YM"] + tachyonDenom x
(αp (n["YM+F^3"] + αp (n["2F^3+F^4"] + αp (n["D^2F^4"] + αp n["(DF)^4"]))))
```

```
Out[48]= n[YM] + 
$$\frac{\alpha p (\alpha p (n[2F^3+F^4] + \alpha p (n[D^2F^4] + \alpha p n[(DF)^4])) + n[YM+F^3])}{1 - \alpha p^2 \sigma_2 - \alpha p^3 \sigma_3}$$

```

And from this, also potentially deformed by a free σ<sub>3</sub>, we have a candidate resummation for what we have found above:

```
In[49]:= expanded = (Normal[Series[n["DF^2+YM"] (1 + αp3 σ3 c[1, 0]), {αp, 0, 4}]] //
Collect[#, {αp}, ExpandAll] & // Collect[#, n[___], FullSimplify] &
```

```
Out[49]= (αp2 + αp4 σ2) n[2F3+F4] + αp3 n[D2F4] + αp4 n[(DF)4] +
(1 + αp3 σ3 c[1, 0]) n[YM] + (αp + αp3 σ2 + αp4 σ3 (1 + c[1, 0])) n[YM+F3]
```

```
In[50]:= ours = nFactorizingAnsatzThrough4 /. fivePointConstraints //
Collect[#, {n[___], αp}, FullSimplify] &
```

```
Out[50]= (αp2 + αp4 σ2) n[2F3+F4] + αp3 n[D2F4] + αp4 n[(DF)41] + αp4 n[(DF)42] +
(1 + αp3 σ3 a[3, YM]) n[YM] + (αp + αp3 σ2 + αp4 σ3 (1 + a[3, YM])) n[YM+F3]
```

```
In[51]:= expanded - ours /. { $\sigma_2 \rightarrow \sigma_{2eval}$ ,  $\sigma_3 \rightarrow \sigma_{3eval}$ ,  $n \rightarrow neval$ } // basisFour // Together //
      easyBasisSolve // List // Last
```

```
Out[51]= {a[3, YM]  $\rightarrow$  c[1, 0]}
```

We see that we line up exactly with our candidate ansatz for resummation.
